# Supplementary material for: A Resource-Free Evaluation Metric for Cross-Lingual Word Embeddings Based on Graph Modularity
Source: arXiv:1906.01926 source file (2019-06-05)
Supplement: Supplementary file 1 [file appendix.tex]

\newpage
\appendix
\section{Seed Words}
\label{appendix:seed_words}

Table~\ref{tab:seed_words} shows the seed words we use to retrieve disaster-related documents in languages other than English in Section~\ref{sec:task2}. 

\begin{table}[h]
\centering
\caption{\label{tab:seed_words}Seed Words}
 \begin{tabular}{llr}
  \hline
  criminality &  sinkholes          \\
  terrorism   &  blizzard           \\
  war         &  drought            \\
  fire        &  hailstorm          \\
  avalanche   &  tornado            \\
  earthquake  &  flood              \\
  lahar       &  wildfire           \\
  landslide   &  disease            \\
 %Coastal erosion         \\
 %Volcanic eruption       \\
 %Heat wave               \\
 %Cyclonic storm          \\
 %Ice storm               \\
 %Climate change          \\
 %Geomagnetic storm       \\
 %Water spout             \\
 %Civil disorder          \\
 %Industrial hazards      \\
 %Engineering hazards     \\
 %Waste disposal          \\
 %Power outage            \\
 \hline
 \end{tabular}
\end{table}

%\section{Linear Regression Fitting}
%\label{appendix:regression}
%In Section~\ref{sec:ablation}, we model: $y = \beta_0 + \beta_1 x_1 + \beta_2 x_2 +  \beta_3 x_3 + \epsilon$,
%where $y$ is the cross-lingual classification accuracy on the Reuters
%corpus, $\beta_i$ are model parameters, $x_1$ is the modularity, $x_2$
%is the \textsc{qvec-cca} score, $x_3$ is the average cosine similarity
%of translation pairs, and $\epsilon$ is the error term. 
%% All input features are standardized before fitting.
%All input features are standardized (zero mean, unit variance) before fitting. 
